# Supplementary material for: Finding undetected protein associations in cell signaling by belief propagation
Source: arXiv:1101.4573 source file (2011-01-24)
Supplement: Supplementary file 1 [file si.pdf]

# Finding undetected protein associations in cell signaling by belief propagation
## *Online Supplementary Information*

Bailly-Bechet M.[1], Borgs C.[2], Braunstein A.[3,4], Chayes J.[2], Dagkessamanskaia A.[5], François J.-M.[5] & Zecchina R.[4,3]

[1] LBBE, CNRS UMR 5558, Université Lyon 1, Villeurbanne, France
[2] Microsoft Research New England, Cambridge, USA
[3] Collegio Carlo Alberto, Via Real Collegio 30, 10024 Moncalieri (TO), Italy
[4] Politecnico di Torino, Torino, Italy
[5] Université of Toulouse, UMR CNRS-INSA 5504 & INRA 792, , Toulouse, France

# 1 Algorithm design

## 1.1 The model

We have mapped the problem of uncovering useful information about signaling pathways on the following constrained minimization task:

$$\min_{\substack{E' \subset E, V' \subset V \\ (E',V')\text{ connected}}} \sum_{e\in E'} c_e - \lambda \sum_{i\in V'} b_i \qquad (1)$$

where $G = (V, E)$ is the graph of protein interactions, prizes $b_i$ represent the differential expression of the gene in the signaling process ($b_i = -\log p_i$ where $p_i$ is the $p$-value of the differential expression) and costs $c_e$ are positive and inversely proportional to the confidence in edge existence. The parameter $\lambda$ regulates the tradeoff between the edge costs and vertices prizes, and

its value indirectly determines the size of the subgraph $G'$. It is easy to see that an optimal subgraph is necessarily a tree and hence that the search can be restricted to trees. In turn trees can be represented through the following pointer/depth representation.

We start with the graph $G = (V, E)$ and a selected *root* node $r \in V$. To each vertex $i \in V$ we will associate a pair of variables $(p_i, d_i)$ where $p_i \in V\ (i) \cup \{*\}$. Here $\partial i = \{j \in V : (i, j) \in E\}$ denotes the set of neighbors of $i$ in $G$, and $d_i \in \{1, \ldots, D\}$. We will denote by $\mathbf{p}$ and $\mathbf{d}$ the vectors $\{p_i\}_{i \in V}$ and $\{d_i\}_{i \in V}$. Variable $p_i$ will denote the ancestor of $i$ in the tree, where the special value $p_i = *$ means that $i \notin V'$, and the auxiliary variable $d_i$ will denote its distance to the root node in the tree (i.e. the *depth* of $i$). In order for variables $\mathbf{d}, \mathbf{p}$ to describe a tree, some constraints should be satisfied:

(a) Depth/time decreases along the tree in direction to the root, i.e. $p_i = j \Rightarrow d_i = d_j + 1$

(b) Nodes that do not participate to the tree ($p_i = *$) should not be parent of some other node, i.e. $p_i = j \Rightarrow p_j \neq *$.

Note that even though the vector $\mathbf{d}$ is redundant (as it can be computed from $\mathbf{p}$), it is crucial to maintain the "locality" of the constraints. For every ordered couple $i, j$ such that $(ij) \in E$, we will define (in the following $\delta$ is the Kroenecker delta)

$$f_{ij}\left(p_i, d_i, p_j, d_j\right) = 1_{p_i = j \Rightarrow d_i = d_j + 1 \wedge p_j \neq *} = 1 - \delta_{p_i, j}\left(1 - \delta_{d_i, d_j + 1}(1 - \delta_{p_j, *})\right) \tag{2}$$

The condition of the subgraph to be a tree will be ensured by imposing that $g_{ij} = f_{ij} f_{ji}$ has to be equal to one for each edge $(ij) \in E$. By extending the definition of $c_{ij}$ by $c_{i*} = \lambda b_i$, then (except for an irrelevant constant additive term), the minimum in Eq. 1 equals to:

$$\min\left\{\mathcal{H}(\mathbf{d}, \mathbf{p}) : (\mathbf{d}, \mathbf{p}) \in \mathcal{T}\right\} \tag{3}$$

where $\mathcal{H}(\mathbf{d}, \mathbf{p}) \equiv \sum_{i \in V} c_{ip_i}$ and $\mathcal{T} = \{(\mathbf{d}, \mathbf{p}) : g_{ij}(p_i, d_i, p_j, d_j) = 1\, \forall (ij) \in E)$.

## 1.2 Derivation of the message-passing cavity equations

Our algorithmic scheme originates from the cavity method of statistical physics, a technique which is known in other fields under different names, namely Belief Propagation (BP), Max-Sum or Sum-Product equations. A recent review can be found in [1].

The starting point is the Boltzmann-Gibbs distribution, which equals to:

$$P(\mathbf{d},\mathbf{p}) = \frac{\exp(-\beta\mathcal{H}(\mathbf{d},\mathbf{p}))}{Z_\beta} \tag{4}$$

where $(\mathbf{d},\mathbf{p}) \in \mathcal{T}$, $\beta$ is a positive parameter (called the inverse temperature), and $Z_\beta$ is the normalization constant (called partition function). In the limit $\beta \to \infty$ this probability concentrate on the configurations of minimum $\mathcal{H}$. See e.g. [1] for a general discussion. The BP approximation consists in a weak correlation assumption between certain probability distributions of single $p_i, d_i$ called "cavity marginals". Given $i, j \in V$, the cavity marginal $P_{j\to i}(d_j, p_j)$ is defined as the marginal distribution $\sum_{(d_k,p_k)_{k\in V\setminus\{j\}}} P_{G^{(i)}}(\mathbf{d},\mathbf{p})$ on a graph $G^{(i)}$ from which node $i$ has been temporally removed. The BP assumption consists in that cavity marginals satisfy the following closed set of equations:

$$P_{j\to i}(d_j, p_j) \quad\propto\quad e^{-\beta c_{jp_j}} \prod_{k\in\partial j\setminus i} Q_{k\to j}(d_j, p_j) \tag{5}$$

$$Q_{k\to j}(d_j, p_j) \quad=\quad \sum_{d_k}\sum_{p_k} P_{k\to j}(d_k, p_k)\, g_{jk}(d_k, p_k, d_j, p_j\} \tag{6}$$

Eqs. 5-6 can be seen as fixed point equations, and solutions are normally searched through iteration: giving a time index $t+1$ and $t$ to the cavity marginals in respectively the left and right sides of Eqs. 5-6, this system is iterated until numerical convergence. Cavity marginals are often called "messages" because they can be thought of as bits of information that flow between edges of the graph during time in this iteration.

## 1.3 Max-sum: $\beta \to \infty$ limit

In order to take the $\beta \to \infty$ limit, Eq. 6 can be rewritten in terms of "cavity fields"

$$\psi_{j\to i}(d_j,p_j) = \beta^{-1}\log P_{j\to i}(d_j,p_j) \tag{7}$$

$$\phi_{k\to j}(d_j,p_j) = \beta^{-1}\log Q_{k\to j}(d_j,p_j) \tag{8}$$

The BP equations (6) in the $\beta \to \infty$ limit take the so-called Max-sum form:

$$\psi_{j\to i}(d_j,p_j) = -c_{jp_j} + \sum_{k\in\partial j\setminus i}\phi_{k\to j}(d_j,p_j) + ct. \tag{9}$$

$$\phi_{k\to j}(d_j,p_j) = \max_{p_k,d_k:g_{jk}\{d_k,p_k,d_j,p_j)=1}\psi_{k\to j}(d_j,p_j\} + ct. \tag{10}$$

Computing the right side of Eq. 10 is in general too costly in computational terms. Fortunately, the computation can be carried efficiently by breaking up the set over which the max is computed into smaller (possibly overlapping) subsets. We define

$$A^d_{k\to j} = \max_{p_k\neq j,*}\psi_{k\to j}(d,p_k) \tag{11}$$

$$B^d_{k\to j} = \psi_{k\to j}(d,*) \tag{12}$$

$$C^d_{k\to j} = \psi_{k\to j}(d,j) \tag{13}$$

In terms of $A, B, C$, Eqs 11-13 and Eqs. 9-10 imply the following equalities:

$$A^d_{j\to i} = \sum_{k\in\partial j\setminus i}E^d_{k\to j} + \max_{k\in\partial i\setminus j}\left\{-c_{jk} - E^d_{k\to j} + A^{d-1}_{k\to j}\right\} \tag{14}$$

$$B_{j\to i} = -c_{j*} + \sum_{k\in\partial j\setminus i}D_{k\to j} \tag{15}$$

$$C^d_{j\to i} = -c_{ji} + \sum_{k\in\partial j\setminus i}E^d_{k\to j} \tag{16}$$

$$D_{j\to i} = \max\left\{\max_d A^d_{j\to i}, B_{j\to i}\right\} \tag{17}$$

$$E^d_{j\to i} = \max\left\{C^{d+1}_{j\to i}, D_{j\to i}\right\} \tag{18}$$

The computation of the right side of Eqs 14-18 can be carried in a time per edge proportional to the depth bound $D$.

## 1.4 Fields

In order to identify the minimum cost configurations, we need to compute the complete (non-cavity) fields, i.e. the fields for the complete graph in which no node has been removed. Given cavity fields, the total fields $\psi_j\left(d_j, p_j\right) = \lim_{\beta\to\infty} \beta^{-1} \log P_j\left(d_j, p_j\right)$ can be written as:

$$\psi_j\left(d_j, p_j\right) = -c_{jp_j} + \sum_{k\in\partial j} \phi_{k\to j}\left(d_j, p_j\right) \quad (19)$$

In terms of the above quantities we find $\psi_j\left(d_j, i\right) = F^d_{j\to i} \stackrel{def}{=} \sum_{k\in\partial j} E^d_{k\to j} + \left(-c_{ij} - E^d_{j\to i} + A^{d-1}_{j\to i}\right)$ if $i \in \partial j$ and $\psi_j\left(d_j, *\right) = G_j \stackrel{def}{=} -c_{j*} + \sum_{k\in\partial j} D_{k\to j}$.

## 1.5 Iterative dynamics and reinforcement

Eqs. 14-18 can be thought as a fixed-point equation in a high dimensional euclidean space. This equation could be solved by repeated iteration of the following dynamical system on $A$,$B$, and $C$ starting from an arbitrary initial condition:

$$A^d_{j\to i}\left(t+1\right) = \sum_{k\in\partial j\setminus i} E^d_{k\to j}\left(t\right) + \max_{k\in\partial j\setminus i}\left\{-c_{jk} - E^d_{k\to j}\left(t\right) + A^{d-1}_{k\to j}\left(t\right)\right\} \quad (20)$$

$$B_{j\to i}\left(t+1\right) = -c_{j*} + \sum_{k\in\partial j\setminus i} D_{k\to j}\left(t\right) \quad (21)$$

$$C^d_{j\to i}\left(t+1\right) = -c_{ji} + \sum_{k\in\partial j\setminus i} E^d_{k\to j}\left(t\right) \quad (22)$$

$$D_{j\to i}\left(t\right) = \max\left\{\max_d A^d_{j\to i}\left(t\right), B_{j\to i}\left(t\right)\right\} \quad (23)$$

$$E^d_{j\to i}\left(t\right) = \max\left\{C^{d+1}_{j\to i}\left(t\right), D_{j\to i}\left(t\right)\right\} \quad (24)$$

These quantities can be thought as messages sent from node $k$ to node $j$ whose meaning is the cost shift that node $k$ communicates to node $j$ of a set of scenarios, respectively:

- $A^d_{k\to j}$ "$j$ points to $k$ at depth $d$"

- $B_{k\to j}$ "$k$ does not belong to the tree"
- $C^d_{k\to j}$ "$k$ points to $j$ at depth $d$"
- $D_{k\to j}$ "$k$ does not point to $j$"
- $E^d_{k\to j}$ "$j$ does not point to $k$ at depth $d$"

This system converges in many cases. When it does not converge, a technique called *reinforcement* is of help [2]. The idea is to perturbate the right side of Eqs. 9 and 19 by adding the term $\gamma_t \psi_i^t(d_i, p_i)$ for a (generally small) scalar factor $\gamma_t$. The resulting equations become:

$$
\begin{aligned}
A^d_{j\to i}(t+1) &= \sum_{k\in\partial j\setminus i} E^d_{k\to j}(t) + \max_{k\in\partial j\setminus i}\left\{-c_{jk} - E^d_{k\to j}(t) + A^{d-1}_{k\to j}(t) + \gamma_t F^d_{j\to k}(t)\right\} && (25)\\
B_{j\to i}(t+1) &= -c_{j*} + \sum_{k\in\partial j\setminus i} D_{k\to j}(t) + \gamma_t G_j(t) && (26)\\
C^d_{j\to i}(t+1) &= -c_{ji} + \sum_{k\in\partial j\setminus i} E^d_{k\to j}(t) + \gamma_t F^d_{j\to i}(t) && (27)\\
D_{j\to i}(t) &= \max\left\{\max_d A^d_{j\to i}(t), B_{j\to i}(t)\right\} && (28)\\
E^d_{j\to i}(t) &= \max\left\{C^{d+1}_{j\to i}(t), D_{j\to i}(t)\right\} && (29)\\
G_j(t+1) &= -c_{j*} + \sum_{k\in\partial j} D_{k\to j}(t) + \gamma_t G_j(t) && (30)\\
F^d_{j\to i}(t+1) &= \sum_{k\in\partial j} E^d_{k\to j}(t) + \left(-c_{ji} - E^d_{i\to j}(t) + A^{d-1}_{i\to j}(t)\right) + \gamma_t F^d_{j\to i}(t) && (31)
\end{aligned}
$$

A C++ implementation of these equations can be found (in source form) on [3].

## 1.6 A note on directness

Note that the cost matrix $(c_{ij})$ needs not to be symmetric, and the same scheme could be used for directed graphs (using $c_{ji} = \infty$ if $(i,j) \in E$ but $(j,i) \notin E$).

## 1.7 Rooting and unrooted trees

On problems on which no root node can be chosen *a priori*, a modified procedure can be used to find unrooted trees (specifically, to find a good root candidate).

In the simple case in which the problem contains a vertex $r$ with a sufficiently large prize such that $r \in T$ if $T$ is an optimal subtree (e.g. $b_r > \sum_e w_e$), then $r$ can be chosen as root. When no such vertex is available, one possible strategy could consist in computing the rooted minimum tree for every possible root, and then choosing the minimum among them. This unfortunately adds a factor $|V|$ to the computational time.

The unrooted minimum can be found more efficiently with the following construction: add an extra vertex $r$ connected to every node on the graph with a (large) edge cost $L$. That is, consider the graph $G' = (V \cup \{r\}, E \cup V \times \{r\})$ where $c_{ir} = L$. Consider the sequence of all subtrees of $G'$: $T_0, T_1...$ ordered increasingly by the cost function $\mathcal{H}'$ defined on $G'$. For $L$ large enough, it is easy to see that the minimum $T_0$ of $\mathcal{H}'$ is the empty graph, the next elements are all trees $T$ with only one link $rs$ to $r$, and thus with cost $\mathcal{H}'(T) = \mathcal{H}(T \cap G) + L < 2L$, followed by all trees with two or more links to $r$, with cost $\mathcal{H}' > 2L$. Trees with only one link to $r$ are in one-to-one correspondence with trees on the original graph rooted on an arbitrary vertex, i.e. "unrooted" trees. We are interested on the *second* minimum, i.e. the tree with exactly one link to $r$ of minimum cost, or equivalently the tree of minimum cost, once the empty graph was excluded. The only vertex $s$ connected to $r$ in this tree can be found by running Max-Sum on $G'$, and then choosing the vertex $s$ for which $F^1_{s \to r}$ is maximum. Afterwards, a second run of Max-Sum on $G$ can be used to find the minimum subtree of $G$ rooted on $s$.

## 2 Numerical results on benchmark problems

While in [4] it has been shown that for random graphs the performance of the algorithm are compatible with known rigorous results, the performances of the algorithm on structured graphs has to be evaluated over benchmark problems. In this respect we have run a systematic check of the performance of the algorithm over the SteinLib database, a renowned benchmark repository of minimum Steiner Tree problems [5]. The aim of the SteinLib (http://steinlib.zib.de) is to collect freely available instances of Steiner tree problems in graphs and provide some information about their origins, solubility and characteristics. Communities within Computer Science who actually work on real world problems, such as Operative Research and Integer Programming researcher, refer to SteinLib as a reliable database.

The algorithm was run with various values of $D$ and $\gamma$, though no *ad hoc* preprocessing of the graphs was performed (a step which typically characterizes heuristics for minimum Steiner tree). Results (see Table 1) show that BP was able to improve the cost of almost all unsolved instances (except two). A comparison on a subset of these instances was also done with the algorithm DHEA from [6] linked to the library CPLEX. Both DHEA and the algorithm that produced the best known costs published on the SteinLib are based on an LP relaxation and linked to CPLEX. A comparison on the PUC/bip shows that DHEA+CPLEX (default parameters) is outperformed by the code from [6], giving slightly worse costs in longer times. Also, in two instances it did not output a feasible tree. In summary, our BP-based approach outperforms both LP-based approaches on these instances.

## 3 Data source and results

The expression datasets from pheromone[8] or rapamycin exposition[9] were used to extract $p$-value of differential expression of all genes, which were then transformed in node prizes

| Instance | SteinLib | BP Cost | BP Time (s) |
|---|---|---|---|
| bip42p | 24818 | 24663 | 22.50 |
| bip42u | 237 | 236 | 29.68 |
| bip52p | 24936 | 24598 | 45.49 |
| bip52u | 235 | 234 | 200.18 |
| bip62p | 22959 | 22858 | 47.02 |
| bip62u | 221 | 220 | 52.67 |
| bipa2p | 35905 | 35375 | 120.67 |
| bipa2u | 342 | 338 | 103.79 |
| cc10-2p | 35687 | 35576 | 84.12 |
| cc10-2u | 345 | 343 | 97.53 |
| cc11-2p | 64366 | 63642 | 194.10 |
| cc11-2u | 620 | 616 | 267.23 |
| cc12-2p | 122925 | 121661 | 808.59 |
| cc12-2u | 1197 | 1180 | 695.46 |
| cc3-10p | 12964 | 12841 | 3058.75 |
| cc3-10u | 127 | 126 | 257.40 |
| cc3-11p | 15816 | 15680 | 395.08 |
| cc3-11u | 154 | 153 | 420.32 |
| cc3-12p | 19011 | 18988 | 736.09 |
| cc3-12u | 187 | 186 | 513.59 |
| cc6-3p | 20458 | 20397 | 88.37 |
| cc6-3u | 199 | 197 | 117.22 |
| cc7-3p | 57459 | 57148 | 392.15 |
| cc7-3u | 554 | 553 | 370.10 |
| cc9-2p | 17451 | 17385 | 24.48 |
| cc9-2u | 172 | 169 | 19.32 |
| hc10p | 60679 | 60366 | 178.54 |
| hc10u | 582 | 581 | 165.15 |
| hc11p | 120471 | 119543 | 104.60 |
| hc11u | 1162 | 1154 | 311.21 |
| hc12p | 241286 | 236398 | 943.45 |
| hc12u | 2304 | 2270 | 1096.12 |
| hc9p | 30310 | 30433 | 70.97 |
| hc9u | 292 | 292 | 65.90 |
| i640-311 | 36005 | 35779 | 24.30 |
| i640-312 | 35997 | 35877 | 52.24 |
| i640-313 | 35758 | 35548 | 55.26 |
| i640-314 | 35727 | 35556 | 11.14 |
| i640-315 | 35934 | 35800 | 15.08 |
| w13c29 | 508 | 507 | 81.87 |
| w23c23 | 694 | 692 | 240.91 |

Table 1: BP performance on open (unsolved) benchmarks of the SteinLib library. Results on the SteinLib were obtained by solving a linear programming relaxation with the commercial library CPLEX using a time cutoff of around 9000s on an equivalent processor [7]. The average time used by BP is 306s and the cost was improved in all but the two smallest instances (hc9p and hc9u with 512 nodes). In instance hc9u BP found the same cost of the one present on SteinLib.

.

| Instance | SteinLib | BP Cost | BP Time (s) | DHEA+CPLEX cost | DHEA+CPLEX time |
|---|---|---|---|---|---|
| bip42p | 24818 | 24663 | 22.50 | 24768 | 33744 |
| bip42u | 237 | 236 | 29.68 | 239 | 78763 |
| bip52p | 24936 | 24598 | 45.49 | 24875 | 15733 |
| bip52u | 235 | 234 | 200.18 | 248 | 17751 |
| bip62p | 22959 | 22858 | 47.02 | - | 14006 |
| bip62u | 221 | 220 | 52.67 | 222 | 12809 |
| bipa2p | 35905 | 35375 | 120.67 | - | 10948 |
| bipa2u | 342 | 338 | 103.79 | 345 | 8146 |

Table 2: Comparison between BP and DHEA+CPLEX from [6] on the open instances of the PUC/bip benchmark set. As best results on SteinLib are also based on a Linear programming relaxation and CPLEX[7], we expected results from DHEA+CPLEX to approximately match bounds of the SteinLib. This was not so: DHEA+CPLEX costs are higher in 4 of 8 cases and did not output a feasible tree in two of the remaining cases despite employing substantially more time. Memory usage was high (around 1G) in some cases.

$b_i = -\log(p_i)$.

The PIN was built from the union of the MIPS [10] and DIP [11] datasets, edges were selected as ”confident” or ”non-confident” based on these database annotations, and edge confidences were defined (up to an irrelevant scaling factor) so as to maximize their correlation with previous analyzes from [12]. We inferred networks with $\lambda$ ranging from 0.05 to 0.9, giving a range of average tree sizes going respectively from 1.5 to 612.7 proteins. The root was chosen according to the current biological knowledge of the pheromone and cell wall integrity pathways in yeast; in treated vs untreated experiments, the root was the known membrane receptor acting as a pathway activator, STE2 for the pheromone pathway, and the main activator PKC1 for the cell wall integrity pathway. In datasets comparing expression in a strain with an over-expressed or deleted gene to the wild type, the modified gene was chosen as the root. The rationale behind this choice was to trace as closely as possible the signals emitted from this gene in the signaling network.

A picture of the results of our analysis is given in figure 1. The biological coherence of the

| $\lambda$ | av. number of shared annotations (BP) | av. number of shared annotations (random weighted) | $p$-value | av. number of shared annotations (random) | $p$-value |
|---|---|---|---|---|---|
| 0.05 | 2.825758 | 2.674521 | 0.3268623 | 2.127607 | 0.02737315 |
| 0.1 | 3.467653 | 2.516274 | 4.998213e-05 | 2.192402 | 6.054992e-07 |
| 0.2 | 2.809935 | 2.381442 | 0.0006109813 | 2.117966 | 4.224614e-07 |
| 0.3 | 2.47841 | 2.311981 | 0.04930697 | 2.076665 | 5.190734e-05 |
| 0.4 | 2.514372 | 2.200001 | 0.0001493055 | 2.057731 | 2.883331e-06 |
| 0.5 | 2.231527 | 2.225341 | 0.4579244 | 2.065522 | 0.002717140 |
| 0.6 | 2.386948 | 2.20798 | 0.005639953 | 2.059939 | 4.146902e-05 |
| 0.7 | 2.158124 | 2.201832 | 0.8718731 | 2.071737 | 0.01250235 |
| 0.8 | 2.378390 | 2.183205 | 0.0006044015 | 2.088608 | 1.468968e-05 |
| 0.9 | 2.183687 | 2.190572 | 0.5767696 | 2.069141 | 0.0008742696 |
| 1 | 2.293075 | 2.187501 | 0.008261032 | 2.088162 | 5.462305e-05 |

Table 3: $p$-values associated with the GO Slim terms enrichment between neighbors in the inferred trees (50 runs on each of the 56 datasets).

56 inferred trees was studied using GO Slim annotations. We tested if the number of shared annotations between neighbors was different in the inferred trees and in random trees of the same size and root, generated either at random or with a choice of the edges inversely proportional to their cost $c_e$. Unilateral $t$-test was performed to compare the average of the number of shared annotations in the different runs. The table 3 shows the results, for $\lambda$ values ranging from 0.05 to 0.9. Note that the results are better for relatively low values of $\lambda$, as expected.

## 3.1 Steiner proteins significance

To investigate whether our results about the Steiner proteins were due to some technical bias (i.e. connectivity bias), we did bootstrap experiments by randomizing the expression data on each of the 56 networks, and by running our algorithm on these randomized data. For the 11 proteins found the more often as Steiner proteins in the real data, we compared their frequency of occurrence as Steiner proteins in the real data relative to the randomized dataset; a high value meaning that their status of Steiner protein was a direct consequence of their position in

| Gene name | Protein | Frac. found (real) | Frac. found (random) | Ratio | $k$ | IB |
|---|---|---|---|---|---|---|
| YBR160W | CDC28 | 0.66 | 0.57 | 1.2 | 227 | 15 |
| YDR388W | RVS167 | 0.52 | 0.31 | 1.7 | 121 | 4.9 |
| YHL048W | COS8 | 0.45 | 0.09 | 5.0 | 46 | 0.63 |
| YFL039C | ACT1 | 0.45 | 0.17 | 2.7 | 47 | 1.1 |
| YER118C | SHO1 | 0.43 | 0.06 | 7.0 | 42 | 1.5 |
| YJR091C | JSN1 | 0.43 | 0.44 | 1.0 | 293 | 25 |
| YCL040W | GLK1 | 0.43 | 0.003 | 144 | 6 | 0.25 |
| YBR159W | IFA38 | 0.41 | 0.09 | 4.8 | 101 | 1.9 |
| YGL181W | GTS1 | 0.41 | 0.09 | 4.5 | 43 | 1.5 |
| YPL181W | CTI6 | 0.41 | 0.02 | 20.3 | 26 | 0.26 |
| YMR059W | SEN15 | 0.34 | 0.007 | 47.5 | 57 | 1.4 |

Table 4: Properties of the 11 putative Steiner proteins found the most frequently in $\lambda = 0.2$ datasets. $k$ stands for connectivity and "IB" for in-betweeness (x$10^5$) .

the network and not their biological significance. Table 4 sums up these results. We see that proteins such as CDC28, due to their high connectivity, often occur as Steiner proteins while simply being hubs in the PIN. COS8, on the other side, is 5 times more often found as a Steiner protein in real data than in random experiments, and has an average connectivity, potentially meaning that it is biologically bridging between various pathways.

# 4 Experimental protocols

We made the $\Delta$COS8 strain for this study, by replacing the chromosomal copy of this gene by cos8::LEU2 deletion cassete. For the overexpression study, we cloned COS8 gene in multicopy plasmid pRS426 (with URA3 marker). To obtain double mutants used in this study cos8::LEU2 deleted BY4741 strain was crossed with a strain from YKO collection (ORF::KAN). Resulted diploid was dissected and segregants having KAN and LEU2 markers were selected and used for further experiments.

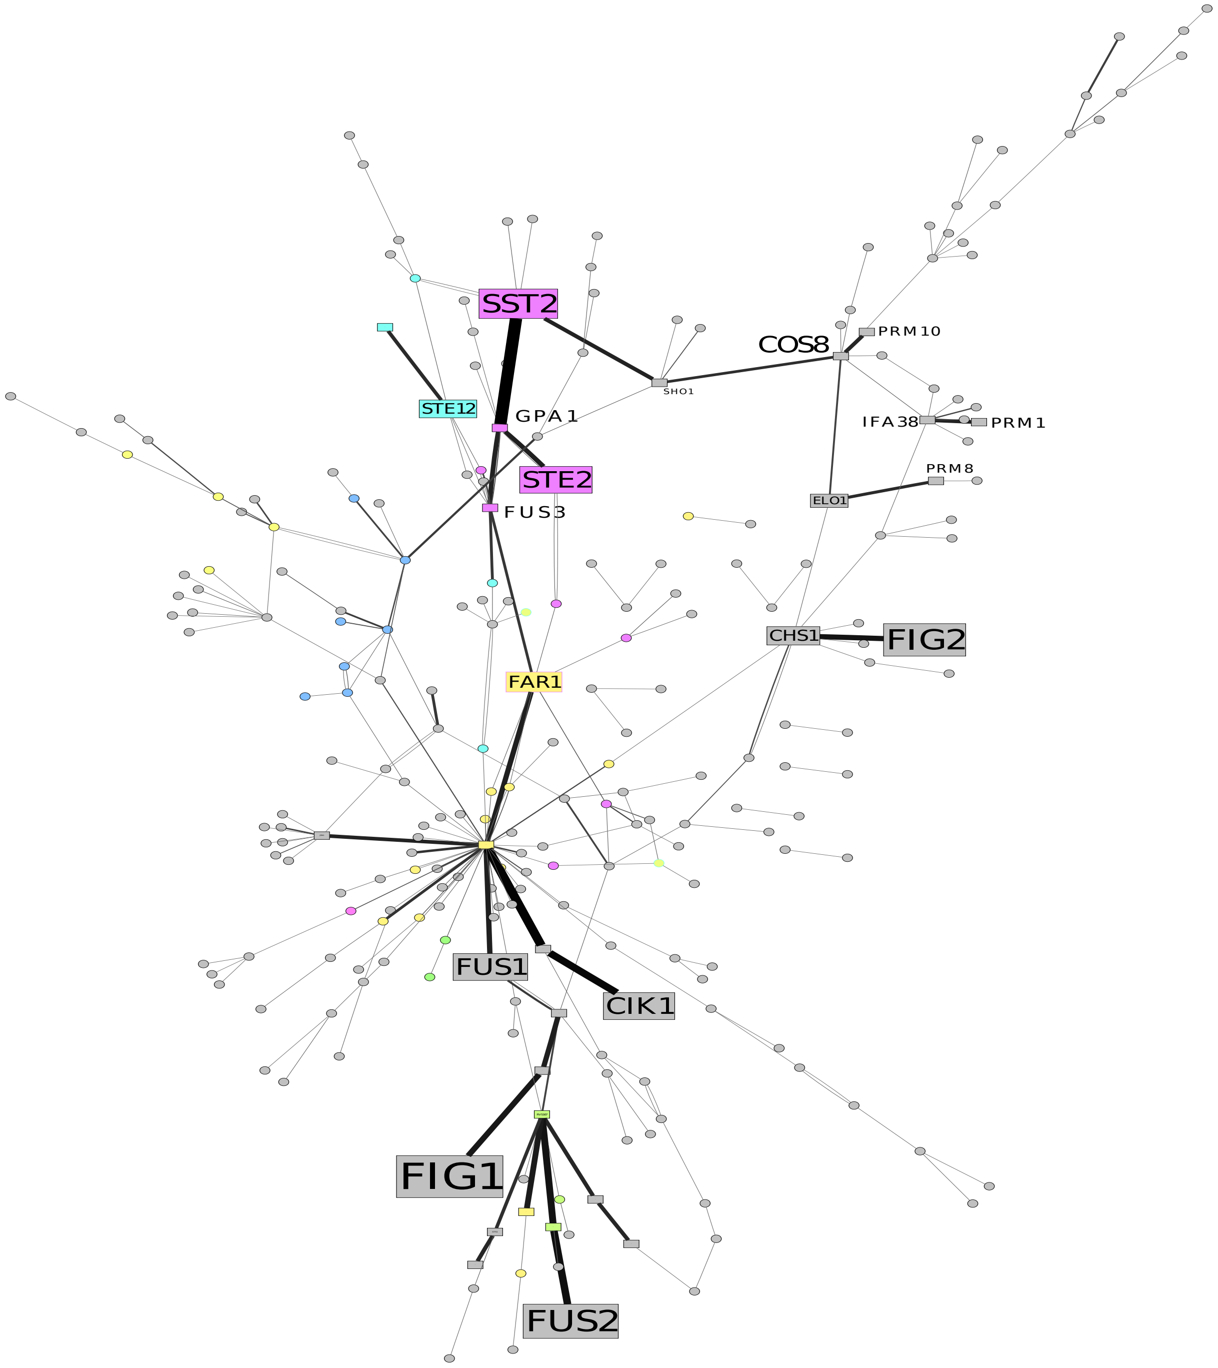


Figure 1: This graph is a subnetwork of the protein-protein interaction map, obtained by including nodes that appear more than 30% of the times on the 56 inferred Steiner trees for $\lambda = 0.2$, with link intensity proportional to the number of times the specific connection was found, and node size proportional to average prize. The layout was decided in order to minimize crossings with the Graphviz suite. Afterwards, colors were added denoting the main GO annotation: Actin (light green), Cell Cycle (yellow), Chromatin structure (blue), Spindle Checkpoint (dark green), Cell wall (cyan) and Pheromone sensing (magenta). The annotations were obtained from the SGD project "Saccharomyces Genome Database" `http://www.yeastgenome.org/`.

## 4.1 Strains, media and culture conditions

BY4741 (MAT a his3-1 leu2-0 ura3-0 met15-0) and relevant deletant strains in this BY background purchased from OpenBiosystem (http://www.openbiosystems.com/YKO) were used as recipient strains for various gene constructs. Yeast transformation was performed according to the lithium acetate method as described in [13]. Yeast cells were cultured in yeast extract (1%), bacto peptone (1%) and glucose (2%) ( YPD), or in yeast nitrogen base (YN) synthetic medium (0.17 % (w/v) yeast nitrogen base without amino acid and without ammonium, supplemented with 0.5% ammonium sulfate (w/v), buffered to pH 4.8 with sodium succinate / NaOH and with the auxotrophic amino acids when required. Cultures were carried out at 30°C in shaking flasks at a shaking speed of 170 rpm/min.

## 4.2 Construction of multicopy plasmid with COS8 chromosomal allele

For amplification of chromosomal copy of COS8 gene we used YGPM 26c13 clone from Yeast Genomic Tiling collection designed by Dr. Greg Prelich (Albert Einstein College of Medicine, see [14]). Primers used for this amplification :

cos8 forward: Xba1TCTAGACAACCATAGTACATAAACACAC
cos8 reverse: Pst1 CTGCAGCA.CATGGCAGTATCTTACC

PCR amplified COS8 fragment was cloned in Xba1 and Pst1 polylinker sites of yeast multicopy vector pRS426 (bears the URA3 marker). Resulted plasmid carrying also URA3 selective marker was used for yeast transformation.

## 4.3 Construction of cos8 deleted strain

The COS8 deletion cassette was made by insertion of BamH1-BamH1 LEU2 gene fragment in BamH1 restriction site of the Xba1-Pst1 COS8 fragment, cloned in pGEMT plasmid. This cassette was then amplified by PCR using the 2 primers, described above (cos8 forward and cos8 reverse), and used for BY4741 and BY4742 strains transformation. Integration of this cassette into genome of the selected clones, growing on YNB leu- plates, were controlled by PCR , using the following primers:

cos8 verif TCACCACTAAAATCACCTAAAC
cos8 reverse: CTGCAGCA.CATGGCAGTATCTTACC

## 4.4 Construction of double mutants

The BY4742 cos8Δ::ΛEY2 strain was crossed with deletion strains from YKO collection (http://www.openbiosystems.com/YKO). After sporulation and tetrads dissection of the resulted diploids, strains carrying cos8::LEU2 allele together with deleted genes with KAN Mx4 cassette was retained for further analysis.

## 4.5 Drug sensitivity assays

The agar Plate sensitivity assays were performed as follows: Strains were grown in liquid media (YPD or YNB-ura minus, when used multicopy plasmids transformants) to exponential phase, then concentrated till DO(600) =8 in sterile water. Two microliters of this cell suspension and its consequent 10 times dilutions were spotted on the solid media with and without drugs, at the concentration indicated in the legends. The plates were scored after two days at 30°C.

# 5 Algorithm comparison with previous data

In order to validate our methodology, we ran our algorithm on a dataset previously studied in [15]. In this study, the authors infer linear signaling pathways of fixed depth, between two fixed proteins. They use a color-coding strategy, and their optimization criterion is more restricted than ours, as they try to minimize only the relative sum of the costs of all edges of their pathway. The results found are summed up in Fig 2, taken from their paper [15].

Here we graphically present our results (see Fig 3), on the same network and using the same set of costs $c_e$. As our algorithm includes node prizes and allows for a bounded but variable depth, we used an uniform prize $b$ for all nodes of the network, and changed this prize from simulation to simulation in order to allow for a variability in the total tree size – which was bounded to 9, as the pathway length was fixed to 9 in [15]. Moreover, our results are trees instead of linear chains, but they are easily comparable with panel (c) of Fig 2. As one can see, as the node prize $b$ increases (in absolute value) the Steiner tree becomes bigger and finally includes almost all relevant proteins of the pheromone pathway, and only them.

In this comparison, we established **(i)** that our methodology, when applied to an already studied dataset, is able to recover precisely the same results, while in a shorter time, due to the fact that the computational cost does grow only linearly with the chain length and not exponentially as in [15] and **(ii)** that these results do correspond to the known biology of the pheromone pathway as schematized in Fig 2 a). On the very short trees as those found here and in [15], the objective is to check the ability of the algorithm to recover the skeleton of known pathways, an essential step to interpret correctly the additional proteins that are added to this skeleton by later analyzes.

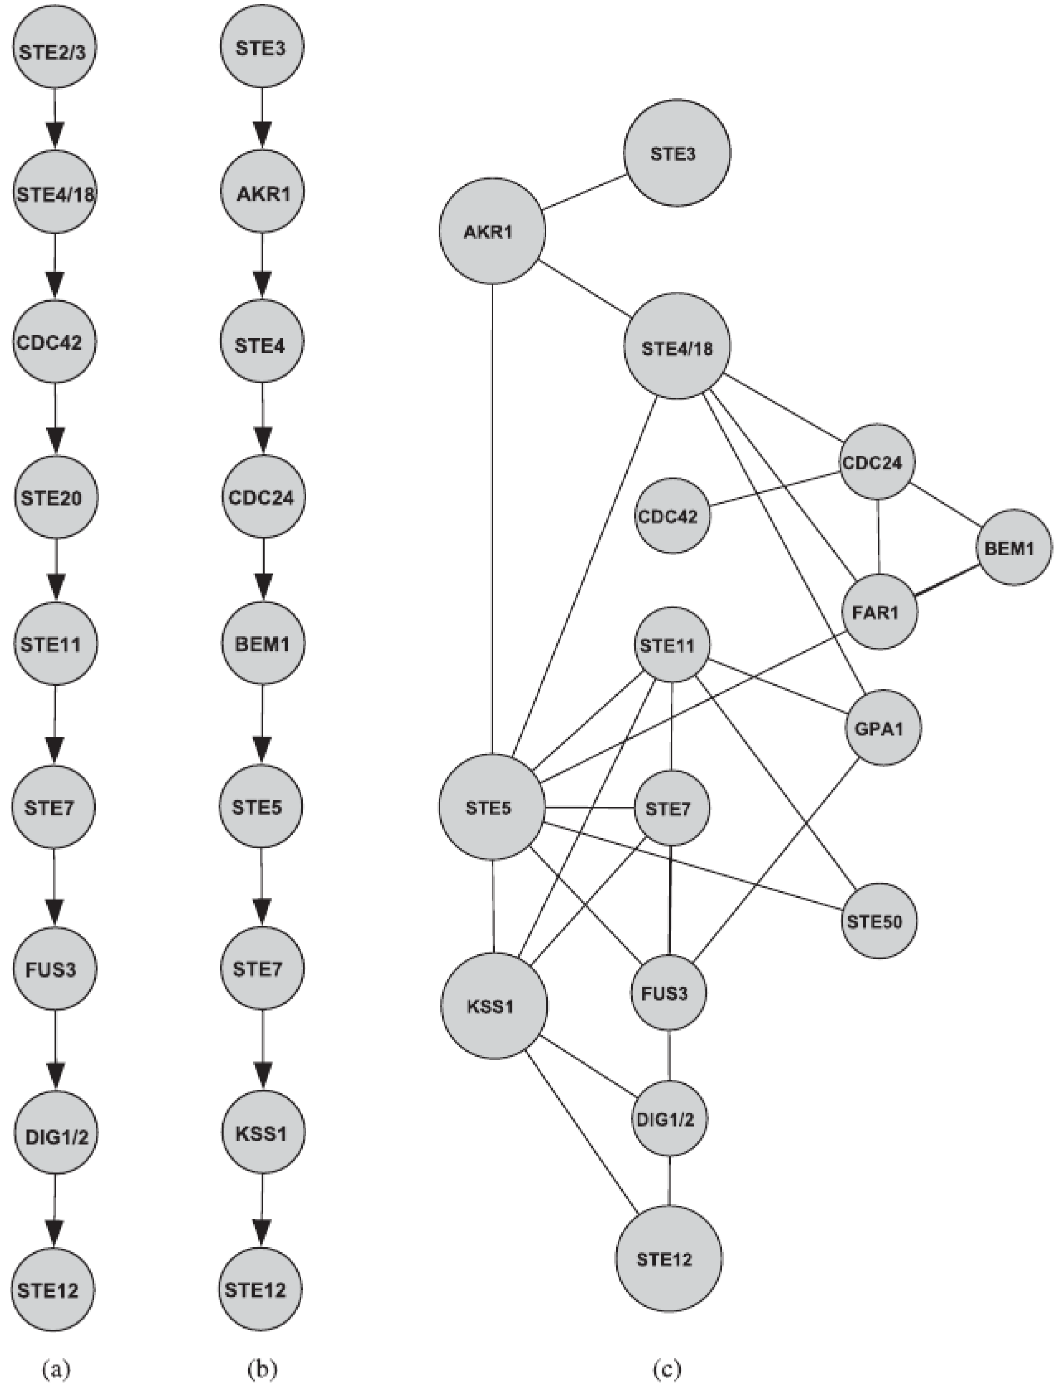


Figure 2: a) the reference yeast pheromone pathway from [8]; b) the best pathway of depth 9 found in the paper; c) the superposition of all pathways found by the color-coding algorithm, where nodes appearing less than 10% of the time have been removed. Bigger circles mean that the nodes are found in more than 50% of the simulations.

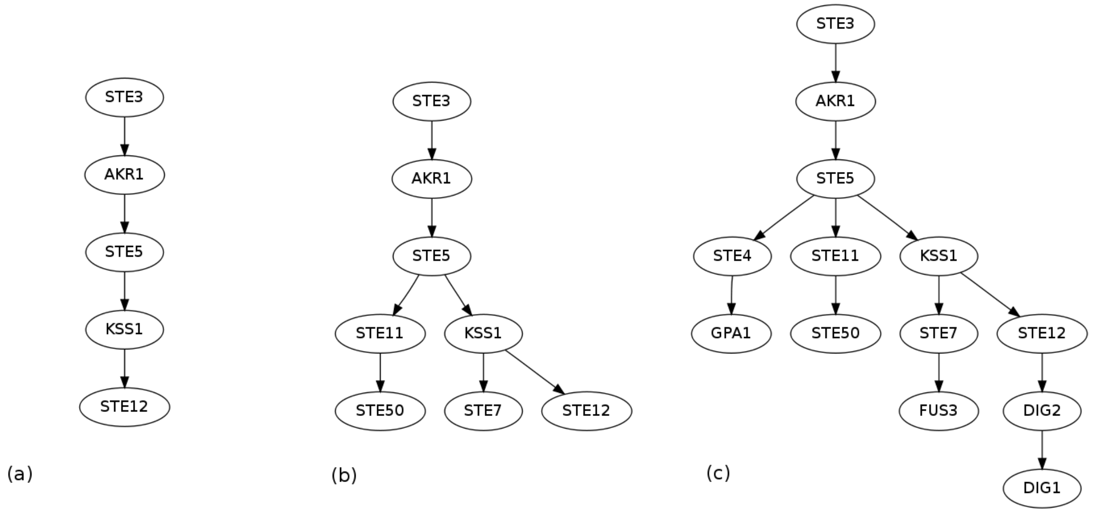


Figure 3: Steiner trees inferred using the same parameters as [15], for different values of the prize $p$ ("lower" prizes tend to increase the tree size, see our optimization criterion). The average edge cost $c_e$ is 0.416; a) $p = 0$, the Steiner tree in this case is the shortest path (for the optimization criterion above) between STE3 and STE12; b) $p = 0.25$; c) $p = 0.255$.

# References

[1] Mezard, M & Montanari, A. (2009) *Information, Physics and Computation*. (Oxford Un. Press).

[2] Braunstein, A & Zecchina, R. (2006) Learning by message-passing in networks of discrete synapses. *Phys. Rev. Lett.* **96**, 030201.

[3] CMP Group, P. d. T. (2010) Cmp website `http://www.polito.it/cmp`.

[4] Bayati, M, Borgs, C, Braunstein, A, Chayes, J, Ramezanpour, A, & Zecchina, R. (2008) Statistical mechanics of steiner trees. *Physical Review Letters* **101**, 37208.

[5] Koch, T, Martin, A, & Voß, S. (2000) SteinLib: An updated library on steiner tree problems in graphs, (Konrad-Zuse-Zentrum für Informationstechnik Berlin, Takustr. 7, Berlin), Technical Report ZIB-Report 00-37.

[6] Ljubić, I, Weiskircher, R, Pferschy, U, Klau, G, Mutzel, P, & Fischetti, M. (2006) An algorithmic framework for the exact solution of the prize-collecting Steiner tree problem. *Mathematical Programming* **105**, 427–449.

[7] Polzin, T. (2003) Ph.D. thesis (Universität des Saarlandes).

[8] Roberts, C. J, Nelson, B, Marton, M. J, Stoughton, R, Meyer, M. R, Bennett, H. A, He, Y. D, Dai, H, Walker, W. L, Hughes, T. R, Tyers, M, Boone, C, & Friend, S. H. (2000) Signaling and circuitry of multiple mapk pathways revealed by a matrix of global gene expression profiles. *Science* **287**, 873–880.

[9] Kuranda, K, Leberre, V, Sokol, S, Palamarczyk, G, & Franois, J. (2006) Investigating the caffeine effects in the yeast saccharomyces cerevisiae brings new insights into the connection between tor, pkc and ras/camp signalling pathways. *Mol Microbiol* **61**, 1147–1166.

[10] Güldener, U, M, M, Oesterheld, M, Pagel, P, Ruepp, A, Mewes, H.-W, & Stümpflen. (2006) Mpact: the mips protein interaction resource on yeast. *Nucleic Acids Res* **34**, D436–D441.

[11] Xenarios, I, Rice, D. W, Salwinski, L, Baron, M. K, Marcotte, E. M, & Eisenberg, D. (2000) Dip: the database of interacting proteins. *Nucleic Acids Res* **28**, 289–291.

[12] Bader, J. S, Chaudhuri, A, Rothberg, J. M, & Chant, J. (2004) Gaining confidence in high-throughput protein interaction networks. *Nat Biotechnol* **22**, 78–85.

[13] RD, W. R. G. (2001) High-efficiency transformation of plasmid dna into yeast. *Methods Mol Biol* **177**, 85–97.

[14] Jones, G. M, Stalker, J, Humphray, S, West, A, Cox, T, Rogers, J, Dunham, I, & Prelich, G. (2008) A systematic library for comprehensive overexpression screens in saccharomyces cerevisiae. *Nat Methods* **5**, 239–241.

[15] Scott, J, Ideker, T, Karp, R. M, & Sharan, R. (2006) Efficient algorithms for detecting signaling pathways in protein interaction networks. *J Comput Biol* **13**, 133–144.
